# Supplementary material for: Model-Based Reinforcement Learning with a Generative Model is Minimax Optimal
Source: arXiv:1906.03804 source file (2020-04-05)
Supplement: Supplementary file 1 [file appendix.tex]

\section{Proofs of supporting Lemmas}

\subsection{Proof of Lemma~\ref{lemma:bounds}}

%\subsection{Proof of Lemma~\ref{lemma:horizon}}

\subsection{Proof of Lemma~\ref{lemma:var_add}}

\subsection{Proof of Lemma~\ref{lemma:crude}}
\label{sec:proof of lemma-crude}

%\subsection{Proof of Lemma~\ref{lemma:cover1}}

%\subsection{Proof of Lemma~\ref{lemma:cover2}}

%\subsection{Proof of Proposition~\ref{prop:cover3}}

%\subsection{Proof of Lemma~\ref{lemma:cover4}}
